# Supplementary material for: A novel trajectory optimization algorithm for continuous-time model predictive control
Source: arXiv:2306.07107 source file (2024-01-23)
Supplement: Supplementary file 1 [file Appendix_A.tex]

\section{Appendix A}
Consider the convex semi-infinite optimization problem 
\begin{equation}
	\label{eq:CSIP_original}
	\begin{aligned}
		& \min_{} && c_{\circ}(x) \\
		& \sbjto && \begin{cases}
			 \overline{h}(x,u) \le 0 \quad \text{for all}\, u\in \mathcal{U},\\
    x \in \mathcal{X},
		\end{cases}
	\end{aligned}
\end{equation}
with the associated data: 
\begin{enumerate}[label=\textup{(\ref{eq:CSIP_original}-\alph*)}, leftmargin=*, widest=b, align=left]
\item\label{csip:data:1} \(\mathcal{X} \subset \Rbb^{n_d}\) is a closed and convex set such that \(\intr \mathcal{X} \neq \emptyset\);
\item\label{csip:data:2} The objective function \(c_{\circ}: \mathcal{X} \lra \Rbb\) is quasi-convex and upper semi-continuous, and the constraint map \(\overline{h}: \mathcal{X}\times \mathcal{U} \lra \Rbb\) is jointly upper semi-continuous in \(x\) and \(u\), and strictly convex in each \(x\) for each fixed \(u\);
\item\label{csip:data:3} \(\intr \mathcal{F} \neq \emptyset\) where \(\mathcal{F}\) is the feasible set defined by \(\mathcal{F} \Let \aset[\big]{x \in \mathcal{X} \mid \overline{h}(x.u) \le 0\,\text{for all}\,u\in \mathcal{U}}\);
\item\label{csip:data:4} The constraint index set \(\mathcal{U}\) is compact. 
\end{enumerate}
To solve the class of optimization problems in \eqref{eq:CSIP_original} a numerically tractable algorithm (which we will call MSA algorithm in the sequel) was provided in \cite{ref:DasAraCheCha-22} under stronger assumptions on the problem data \eqref{csip:data:1}--\eqref{csip:data:4}. Since the MSA algorithm solves a relaxed convex program with a finite constraint index set instead of the infinite index set \(\mathcal{U}\), the set of optimizers obtained thereby is only a priory known to be a superset of the original solutions. When \(c_{\circ}(\cdot)\) is a strictly convex function, the solution of the relaxed optimization problem (see equation (2.7) in \cite{ref:DasAraCheCha-22}) coincides with that of the original optimization problem in the sense that
the optimal values and the optimizers of the relaxed and the original SIP are the same. Let us briefly talk about the chief ideas behind the MSA algorithm. Define a map \(\mathcal{G}: \mathcal{U}^{n_d} \lra \Rbb\) which involved a constraint convex program with a finite index set \(\mathcal{U}^{n_d}\)
\begin{align}
    \mathcal{G}(u_1,\ldots,u_{n_d}) \Let \inf_{x \in \mathcal{X}} \aset[\bigg]{c_{\circ}(x) \mid \overline{h}(x,u_i) \le 0 \quad \text{for}\,i=1,\ldots,n_d}.
\end{align}
It can be shown that under a specialized set of problem data (\(c_{\circ}\) convex and continuous, \(h\) convex in \(x\) and jointly continuous in \(x\) and \(u\)) the optimal value of the semi-infinite program \eqref{eq:CSIP_original} is the same as the optimal value of the global optimization problem 
\begin{align}
\sup_{(u_1,\ldots,u_{n_d}) \in \mathcal{U}^{n_d}} \mathcal{G}(u_1,\ldots,u_{n_d}),
\end{align}
see \cite[Theorem 1]{ref:DasAraCheCha-22}. The primary engine behind the proof of the theorem is \cite[Theorem 4.1]{JMB:81}. An extension of the MSA algorithm --- the MSAP algorithm, has been reported in \cite{ref:ParuCha22} under the data \eqref{csip:data:1}--\eqref{csip:data:4}. The same equivalence result as that of MSA also follows for the MSAP algorithm.
